# Supplementary material for: Magnetic field-tuned superconductor/insulator transition in TiN nanostrips
Source: arXiv:1806.01335 source file (2018-06-04)
Supplement: Supplementary file 1 [file Schneider_supplement_arXiv.pdf]

# Supplementary material for
# Magnetic field-tuned superconductor/insulator transition in TiN nanostrips

I. Schneider[1], K. Kronfeldner[1], T.I. Baturina[1,2], and C. Strunk[1]
[1]*Institute of Experimental and Applied Physics, University of Regensburg, D-93040, Germany and*
[2]*Institute of Semiconductor Physics, 13 Lavrentjev Avenue, Novosibirsk, 630090 Russia*
(Dated: May 15, 2018)

We provide $R(T)$, discuss the thermally activated phase slips at zero magnetic field, the magnetoresistance, and the $I$-$V$-characteristics of wider and narrow strips. The adaptation of the Ivanchenko-Zilberman theory is described in detail together with the systematic dependence of the fit parameters with strip width.

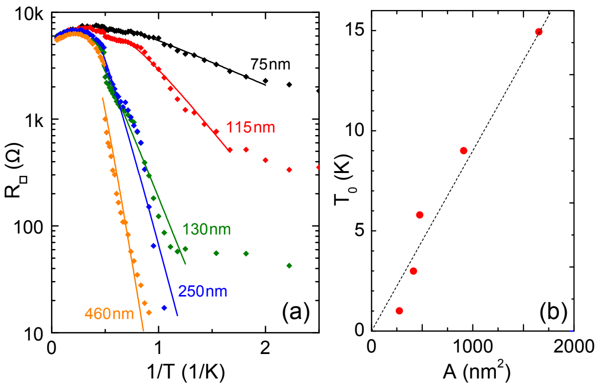


FIG. S1. (a) Arrhenius plot of the resistance at zero magnetic field for different strip width of chip A. The lines are fits according to Eq. S1. The resistance of the narrowest strips saturates at low temperature. The lines are fits according to Eq. S1. (b) Activation temperatures $T_0$ vs. cross section $A = wt$ extracted from the fits in (a). The slope of the dashed line corresponds to an effective Ginzburg-Landau parameter of $\kappa_{\rm eff} \simeq 490$.

## THERMALLY ACTIVATED PHASE SLIPS

In order to understand the temperature dependence of the resistivity at zero magnetic field, we have fitted the data in Fig. 1 using a simplified version of the Langer-Ambegaokar model[1–3] :

$$R(T) \;=\; R_0 \exp(-\Delta F_0(T)/k_{\rm B}T)\;, \qquad \text{(S1)}$$

where $R_0$ is a fixed prefactor, and the activation energy corresponds to the loss of superconducting condensation energy near the mean-field transition temperature, $T_c$,

$$\Delta F_0(T) \;=\; k_{\rm B}T_0 \cdot (1 - T/T_c)^{3/2}\;. \qquad \text{(S2)}$$

The characteristic temperature, $T_0$, of the activation process is given by

$$T_0 \;=\; \frac{\xi_{\sf GL} wt}{k_{\rm B}\mu_0}\left(\frac{\hbar}{4e\kappa\xi_{\sf GL}^2}\right)^2\;, \qquad \text{(S3)}$$

which is controlled near the $T_c$ by the Ginzburg-Landau coherence length $\xi(T) \;=\; \xi_{\sf GL}/\,(1 - T/T_c)^{1/2}$ and the Ginzburg-Landau parameter $\kappa$. The regime of thermally activated resistance is clearly visible in the Arrhenius plot, in Fig. S1a, while the resistance of the narrower strips saturates at gradually increasing resistance levels. Solid lines are fits corresponding to Eq. S1. The activation temperatures extracted from these fits are shown in Fig. S1b, while the prefactors $R_0 \simeq 6.7 \pm 1\,{\rm k}\Omega$ slightly scatter in an interval that contains the quantum resistance $R_Q = 6.45\,{\rm k}\Omega$. We observe a good proportionality between the values of $T_0$ and the strip width, $w$, as expected from Eq. S3. Taking $\xi_{\sf GL} = 8.9\,{\rm nm}$ [4], we can extract an effective Ginzburg-Landau-parameter of $\kappa_{\rm eff} \simeq 490$ from the slope of the interpolation line. This value is a factor 2.5 larger than the $\kappa$-value obtained independently on the same TiN-film [4]. Given the fact, that our strips are considerable wider than the coherence length and very close to the SIT such agreement is very satisfactory. It suggests that the concept of thermally activated phase slips (in our case more phase slip lines [5]) can at least qualitatively be transferred to films substantially wider than the coherence length.

## EFFECT OF MAGNETIC FIELD IN WIDER STRIPS

In Figure S2 we show the effect of magnetic field on the $R(T)$-curves for some of the wider TiN strips both on semilogarithmic scales lg $R$ vs. $T$ (left column) and $R$ vs. lg $T$ (right column). The logarithmic representation of $R$ (left column) shows that for $w = 460\,{\rm nm}$ the transition temperature is gradually suppressed, while the resistance goes to zero for $B \leq 2.6\,{\rm T}$. The resistance $R(T, B = 3\,{\rm T}) \simeq R_N/2$, indicates that the critical magnetic field of the film is close to 3 T. For $w = 250\,{\rm nm}$ and $B \gtrsim 0.4\,{\rm T}$ the magnetic field induces a saturation of $R(T)$ at low temperatures. The saturation level $R_{\rm sat}$ gradually increases with the field. The increasing $R_{\rm sat}$ is again consistent with an increase of the quantum phase slip rate that results from a suppression of the Josephson coupling energy with increasing magnetic field. For $w = 130\,{\rm nm}$ the saturation occurs in zero field already.

The linear representation of the resistance (right column) shows that no insulating reentrance is observed in

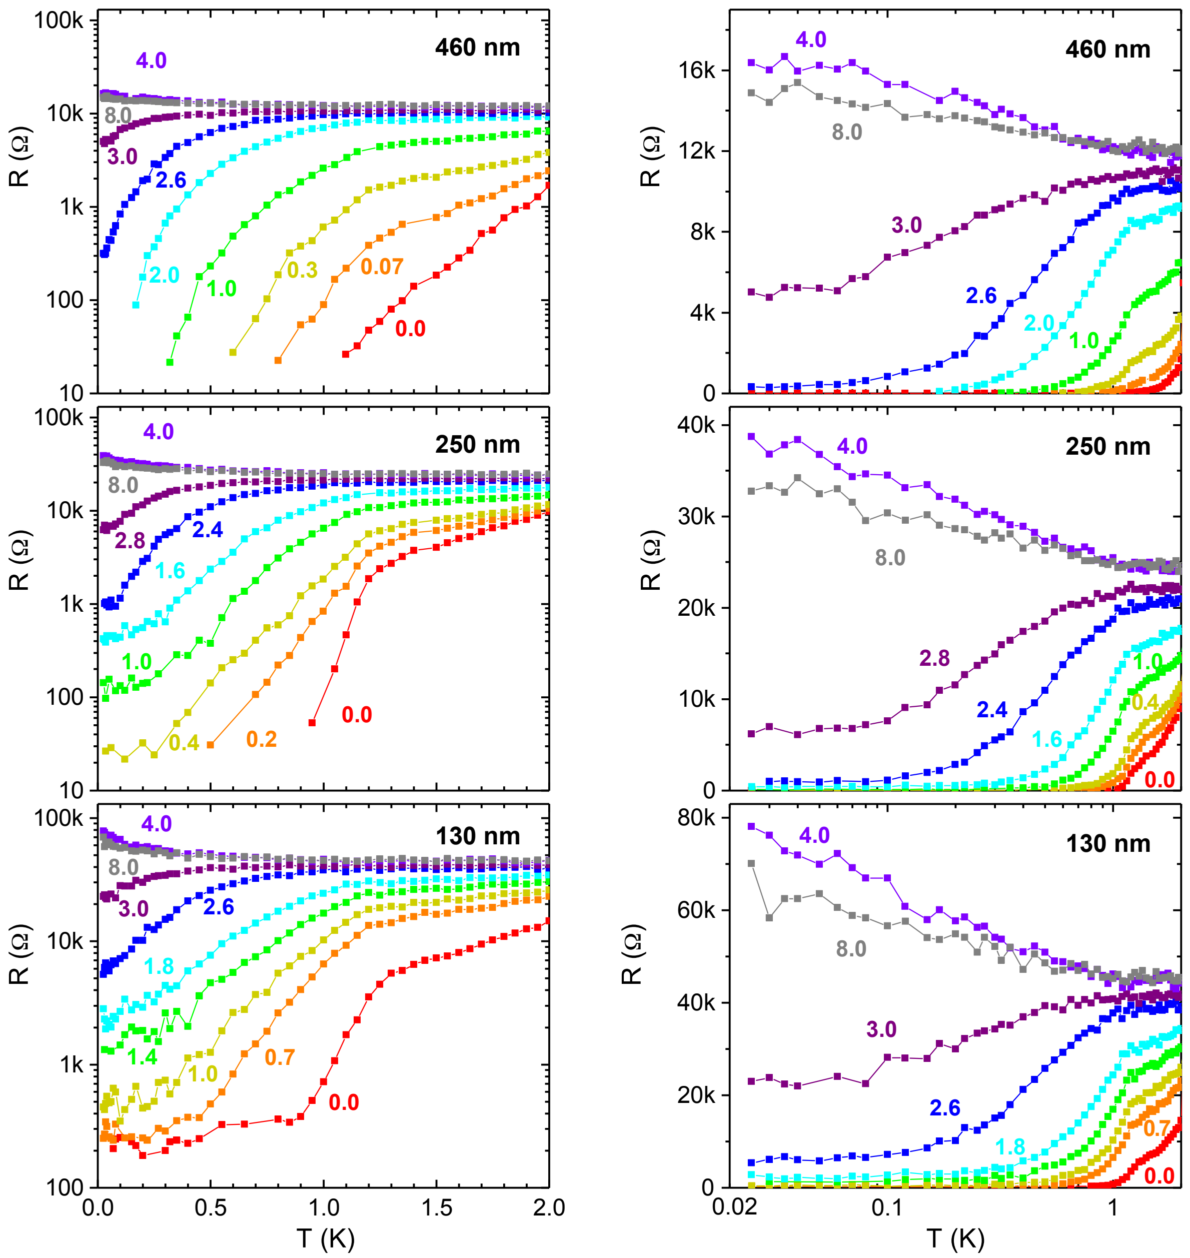


FIG. S2. Resistance vs. temperature in perpendicular magnetic field for the wider TiN strips.

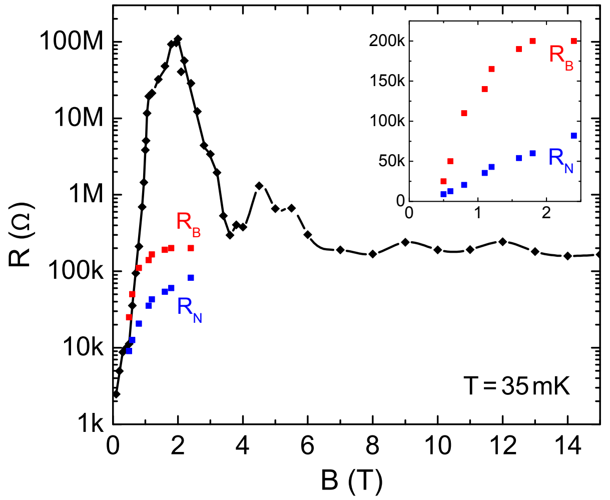


FIG. S3. Magnetoresistance of the wire with $w = 85\,\mathrm{nm}$ (black diamonds). The resistances $R_\mathrm{N} = 1/G_\mathrm{N}$ extracted from the high voltage part of the $I$-$V$-characteristics (blue squares) and $R_\mathrm{B} = 1/G_\mathrm{B}$ from the IZ-fits (red squares) are shown. The inset shows the evolution of the fit parameters $R_N$ and ${}_B$ (see last section).

these devices at any field. This observation supports our view that the reentrant behavior discussed in the main text requires the presence of a dominating weak spot of the sample, where a current blockade occurs that is induced by the proliferation of quantum phase slips. At magnetic fields $B \gtrsim 4\,\mathrm{T}$, that exceeds the critical field of the TiN, $R(T)$ logarithmically rises as expected from the quantum corrections to the resistivity in a strongly disordered metal. For smaller nanostrip width $w < 130\,\mathrm{nm}$ these corrections become quite substantial (80%). It remains, however, much smaller than the resistance increase induced by the Coulomb blockade of Cooper pairs that appears responsible for the reentrant behavior in these devices (see Fig. S3 below). The non-linear resistance of the nanostrip (not shown) in a magnetic field of 5 T can be used, to estimate the relevance of heating effects in the insulating regime. Similar to the data in [6], voltages around 100 $\mu$V at 35 mK are needed for an appreciable heating effect, corresponding to a current of 2 nA and a power input of 0.2 nW. Near the Bloch nose in Fig. 4a in the main text, the power dissipation is about 2 fW, and thus two orders of magnitude smaller. Hence, we can exclude heating effects as the origin of the non-monotonicity in the $I$-$V$-curves in the strongly insulating regime.

## MAGNETORESISTANCE IN NARROW WIRES

Figure S3 displays the low temperature magnetoresistance of the wire with $w = 85\,\mathrm{nm}$. Superimposed on a large peak, the magnetoresistance displays wiggles that remind to the magneto-fingerprints familiar from disordered normal-conducting wires [7]. Such random fluctuations are consistent with fluctuations of the local $E_J$ in our disordered TiN nanostrips ($w < 100\,\mathrm{nm}$). They are expected to cause complex frustration patterns in a random multi-loop topology.

These can also explain the observed fluctuation pattern of $V_c(B)$ (see Fig. 4d in the main text), as the magnetoresistance at the weakest spot is controlled by the combination of a few Josephson loops with random sizes. The characteristic resistances $R_\mathrm{N}$ and $R_\mathrm{B}$ extracted from the $I$-$V$-characteristics are shown as blue and red squares, respectively. As seen in Fig. S6e, both $R_\mathrm{N}$ and $R_\mathrm{B}$ gradually approach the normal state resistance of the wires in the limit of high magnetic field.

## EVOLUTION OF $I$-$V$-CHARACTERISTICS WITH DECREASING STRIP WIDTH

In Fig. S4 we show the evolution of the $I$-$V$-characteristics with increasing wire width. For the narrowest strips the supercurrent peak is very small and rounded. The slope of $I(V)$ remains finite, but decreases with the strip width. The temperature corresponding to the lowest slope in the high voltage regime, i.e., near the temperature of the maximum in $R(T)$ decreases from 4.5 to 2.8 K when $w$ decreases from 800 to 75 nm. This leads to a crossing of the $I$-$V$-characteristics at high voltages for the narrower wires. At a magnetic field of 5 T the differential conductance $dI(V)/dV$ of the narrower strips displays a zero bias anomaly, i.e., a narrow dip around zero bias, similar to observations in MoGe nanowires [6]. The size of the dip is close to the resistance increase below 1 K at such magnetic field (right column in Fig. S2). These comparatively weak nonlinearities are consistent with the temperature dependence of the conductance, if electron heating occurs at elevated voltages. Electron heating is relevant, because the electron phonon coupling in metals becomes so weak at the lowest temperatures that the local electron temperaure in the wire raises above the phonon temperature. The electric power required to significantly change the differential conductance amounts to a fraction of a picowatt – two orders of magnitude larger than the power near the current/voltage peaks in Figs. 2a and 4a in the main text, respectively.

For the wider strips (480 and 800 nm) the form of the $I$-$V$-characteristics changes drastically: after a very sharp peak a shoulder forms in $I(V)$ at a rather high current level, which drops abruptly to a plateau at much lower current around 100-150 $\mu$V and then gradually approaches the normal state resistance. The shoulder is identified as a 'relaxation-oscillation' plateau known from conventional Josephson junctions [8]. It vanishes above $T \gtrsim 1\,\mathrm{K}$ and reflects dynamical oscillations of voltage and

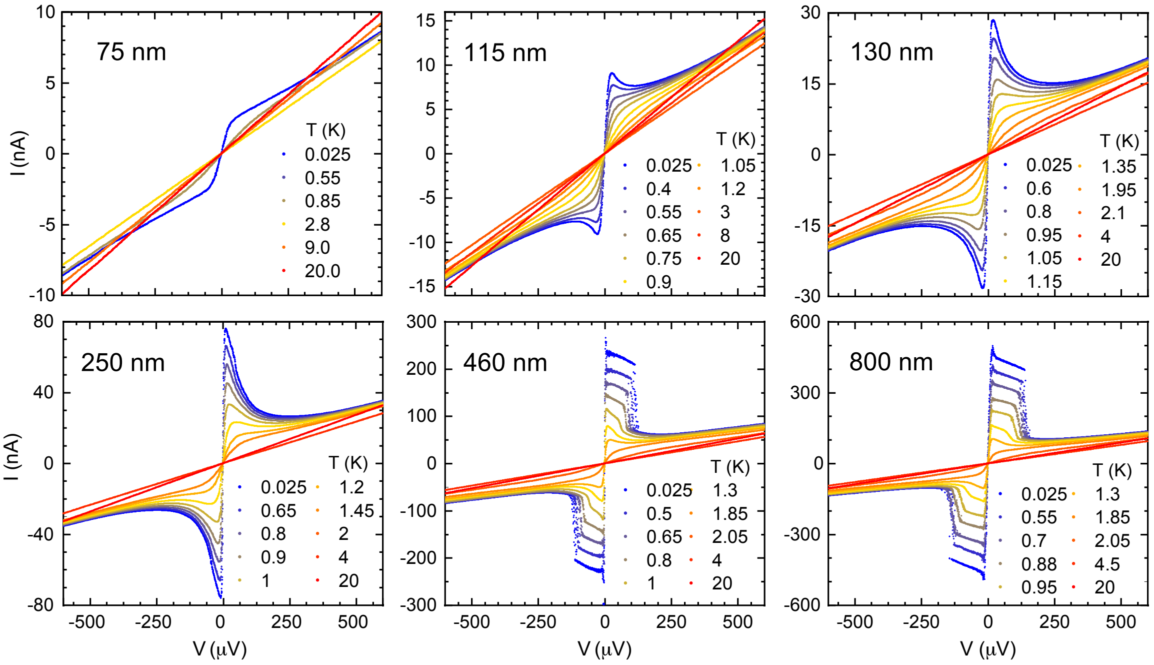


FIG. S4. $I$-$V$-characteristics for different nanostrips width and temperatures in zero magnetic field.

current that are controlled by the time-constants of the $LC$-circuit formed by the sample together with its electromagnetic environment. The lower plateau is followed by gradual approach of $I(V)$ towards the normal state $I$-$V$-characteristics that is typical for the so-called hot spot behavior that is known from superconducting microbridges [9]. Such a combination of relaxation-oscillation and hot-spot behavior is also found for millimeter-sized two-dimensional TiN films [10]. The crossover between the two types of $I$-$V$-characteristics constitutes further evidence that the character of the junctions dynamics drastically changes from microbridge-like towards Josephson-like as the strip widths is reduced.

## SUPERCURRENT PEAK IN NARROW WIRES

We compare our experimental results to an adaption of the Ivanchenko-Zilberman (IZ) model [11], in which the smearing of the critical current with increasing temperature is connected to the Johnson-Nyquist noise of a resistor $R_B$ in series with a small Josephson junction. The current-voltage characteristics in this model reads:

$$I(V_{\rm IZ}) \;=\; I_0\, \Im{\rm m}\left[\frac{\mathcal{J}_{1-\hbar V_{\rm IZ}/2eR_Bk_BT}(\hbar I_0/2ek_BT)}{\mathcal{J}_{-\hbar V_{\rm IZ}/2eR_Bk_BT}(\hbar I_0/2ek_BT)}\right], \tag{S4}$$

where $\mathcal{J}_\nu(z)$ is the modified Bessel function, $V_{\rm IZ} = V + R_B I$ denotes the voltage of the junction connected in series with the bias resistor $R_B$, while $V$ being the voltage across the junction that is measured in our experiment.

Figure S5 shows a comparison of the theory with the supercurrent peaks observed in the four narrowest devices on chip A. The maximal supercurrent differs by more than a factor of 40, while the strip width is changed only by a factor of 4. After subtraction of the current contribution through a parallel resistor $R_N$ (see main text and the discussion below) the supercurrent peaks of all four devices can be fitted within the IZ-theory using Eq. S4, if we model the effect of a finite charging energy $E_C < E_J$ by replacing the bath temperature $T$ with an effective temperature $T_{\rm eff}$. A finite charging energy implies quantum fluctuations of the phase. The phase fluctuations lead to a saturation of the height and width of the supercurrent peak, which is exactly what we observe below $\simeq 350\,$mK. The intrinsic critical current $I_0$ and $T_{\rm eff}$ together determine the height of the supercurrent peak. For a single $I(V)$-trace the fit values of $T_{\rm eff}$ and $I_{c0}$ are dependent on each other. This ambiguity is removed by the demand that $I_{c0}$ should first increase with decreasing $T_{\rm bath}$ and then saturate, while $T_{\rm eff}$ should first decrease and agree with the measured temperature $T$ and then deviate from $T$ and eventually saturate. The resulting values of $I_{c0}$ and $T_{\rm eff}$ are shown in Fig. 2d (main text), and Fig. S6a, respectively. Given our low temperature filtering, the fit-values extracted for $T_{\rm eff}$ at low $T$ are far too large, to be explained by artifacts like residual noise. The saturation of $T_{\rm eff}(w)$ correlates with the saturation of $R(T \to 0, w)$ in Fig. 1 (main text) and is very likely a manifestion of QPS, i.e., small but, finite values of $E_C/E_J$ not captured by the Ivanchenko-Zilberman theory.

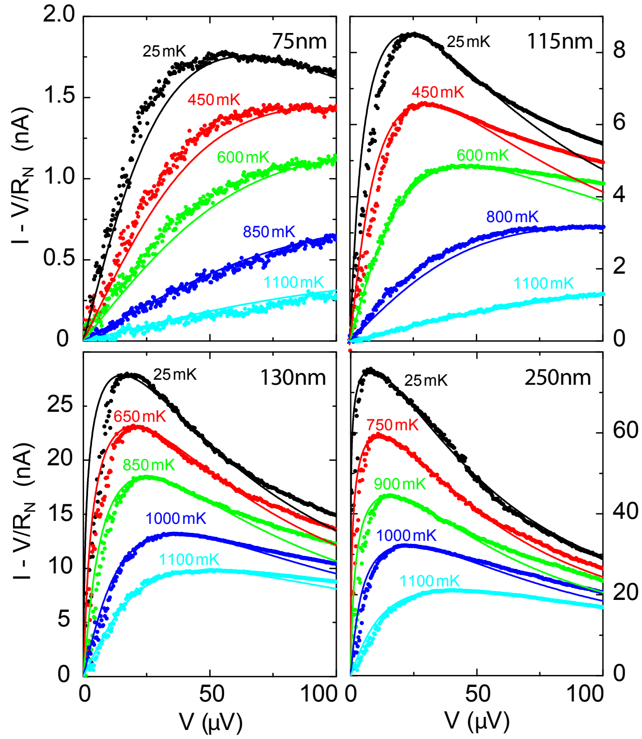


FIG. S5. Supercurrent peaks of the four narrowest wires on chip A. The solid lines are fits according to the Ivanchenko-Zilberman model with $V = V_{\rm IZ} - R_B I$ (see text).

A second adaption of the original IZ-model results from the fact, that the dominating Josephson element in our device is embedded into an electromagnetic environment with a frequency dependent impedance $Z(\omega)$, which is parallel to the active spot. At zero frequency the real part of that impedance is given by Re $Z(\omega = 0) = R_N$, where $R_N$ is determined from the linear part of the $I$-$V$-characteristics at high bias. The physical origin of $R_N$ is most likely a parallel quasiparticle contribution to the current that takes over once the Josephson current is suppressed at high temperatures and voltages. Since $R_N = 0$ in the IZ-model, we need to subtract the contribution $V/R_N$ from the measured current, in order to compare the model and the data. The values of $R_N$ determined independently from the high voltage limit $I$-$V$-characteristics are plotted vs. wire width in Fig. S6b (blue squares). As illustrated at $B = 0$ in Fig. S6c these values correlate very well with the maxima of the $R(T)$-curves for all four samples in Fig. S5.

On the other hand, the lead capacitance effectively short the (high) internal resistance of the voltage source at high frequencies, which renders the parallel and serial connection of $Z(\omega)$ and the sample to be equivalent. Near the plasma frequency $\omega_p$ the real part of $Z(\omega \simeq \omega_p)$ corresponds to the fit parameter $R_B$ in the IZ-formula (Eq. S4). As a source of thermal voltage noise, $R_B$ controls the thermal smearing, i.e., the height and width of the supercurrent peak. In Fig. S6b we show the fit-values of $R_B$ as a function of wire width (red squares). The $R_B$-values mainly affect the current scale above which the $V_{\rm IZ}$ is vanishing in the fits. We find $R_B < R_N$ as expected for an electromagnetic environment with shunting lead capacitances.

## CURRENT BLOCKING AT INTERMEDIATE MAGNETIC FIELDS

In this section, we demonstrate that the behavior in the reentrant insulating regime at finite magnetic field $0.5\,{\rm T} \lesssim B \lesssim 2.4\,{\rm T}$ obeys a strong duality symmetry when compared to the zero field case. A necessary prerequisite for a strong Coulomb blockade is the isolation of the active elements by a high impedance environment. The environment impedance can be either resistive [12–14] or inductive [15–18]. The on-chip leads towards our nanostrips are made from low-resistive gold. Hence, the only candiates for a high-impedance element protecting the active spot of the nanostrips are the more robust sections of the strip adjacent to the active spot. In the superconducting state we estimate the kinetic inductance (using $R_N = 67\,{\rm k}\Omega$ and $T_c \simeq 1.5\,{\rm K}$) to be $L_{\rm kin} \simeq 0.14\hbar R_N/k_B T_c \simeq 380\,{\rm nH}$. With the gradual suppression of superconducting correlations in high magnetic field the large normal state resistance $R_N$ of the nanostrip gradually takes over.

We used the dual version of the IZ-model in the form [17]

$$V(I_{\rm IZ}) = V_0\, \Im{\rm m}\left[\frac{\mathcal{J}_{1-eI_{\rm IZ}/\pi G_B k_B T}(eV_0/\pi k_B T)}{\mathcal{J}_{-eI_{\rm IZ}/\pi G_B k_B T}(eV_0/\pi k_B T)}\right], \quad \text{(S5)}$$

where $I_{\rm IZ} = I + G_B V$ is the current of the junction connected in parallel to the bias conductor $G_B = 1/R_B$, while $I$ denotes the current through the junction that is measured in our experiment. As on the superconducting side, we introduce an effective temperature in order to describe this time the effects of a finite Josephson coupling $E_J < E_C$ and residual noise in the system. An analogous fitting procedure results in values of $V_0$ and $T_{\rm eff}$ that are shown in Fig. 4a (main part), and Fig. S6d, respectively. When compared to their counterpart at the superconducting side (Fig. S6a) the values of $T_{\rm eff}$ are an order of magnitude smaller and do not vary significantly with magnetic field.

Dual to the superconducting side the environmental admittance $Z^{-1}(\omega)$ is now in series with the nanostrip. Analogous to the superconducting case at $B = 0$ the zero frequency limit $Z^{-1}(\omega = 0) = G_N$ is reflected as a linear contribution $I/G_N$ to the $V(I)$-characteristics, which has to be subtracted from the measured voltage. The values of $G_N$ obtained from the high voltage part of the $V(I)$-characteristics are plotted vs. magnetic field

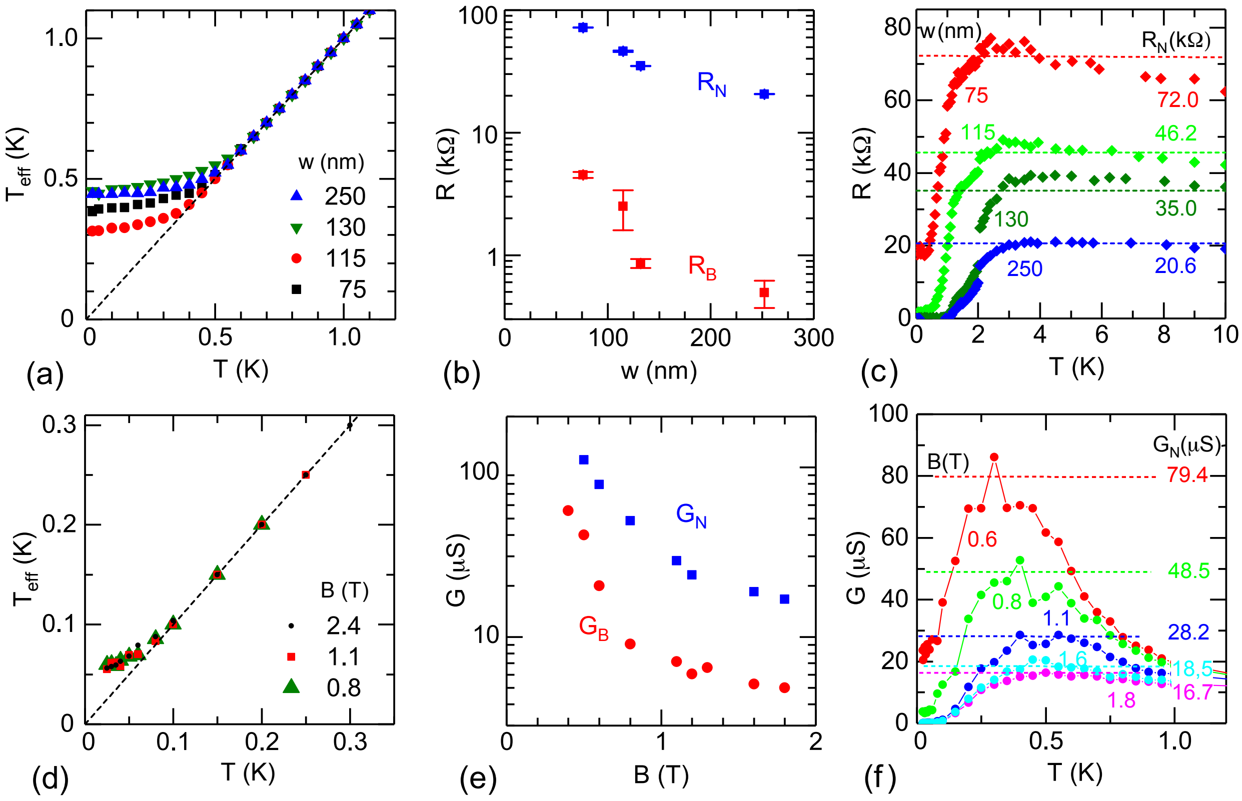


FIG. S6. (a) Effective temperature used in the IZ-analysis of the supercurrent peak of the four narrowest strips at zero magnetic field. The dashes line corresponds to $T = T_{\mathrm{eff}}$. (b) Corresponding fitparameters $R_N$ and $R_B$ extracted from the IZ-analysis. (c) Resistance $R(T)$ of the same samples. The dashed horizontal lines denote the $R_N$-values from (b). (d) Effective temperature used in the dual IZ-analysis of the Bloch nose in the reentrant insulating regime. (e) Corresponding fitparameters $G_N$ and $G_B$ extracted from the dual IZ-analysis. (f) Conductance $G(T)$ in the insulating reentrance observed for the 85 nm wide strip. The dashed horizontal lines denote the $G_N$-values from (e).

(blue circles) in Fig. S6d. Analog to the superconducting side Fig. S6f shows that these values correlate very well with the maxima of the $G(T)$-curves for several values of the magnetic field.

At high frequencies the lead capacitance again shorts the internal resistance of the voltage source. Hence, the parallel and serial connection of $Z(\omega)$ and the sample are equivalent (as on the superconducting side). Near the plasma frequency Re $Z^{-1}(\omega \simeq \omega_p)$ corresponds to the fit parameter $G_B$ in the dual IZ-formula (Eq. S5). Now $G_B$ (red circles) as a source of thermal current noise controls the thermal smearing, i.e., the height and width of the Bloch nose (Fig. 4a, see main text). In Fig. S6e we show the values of $G_B$ determined from the fits together with $G_N$ as a function of magnetic field. It includes a contribution from the two bias resistors ($2 \times 50\mathrm{k}\Omega$) in series with and near to the sample. We find $G_N > G_B$ as expected from the duality to the superconducting side.

Also dual to the resistance $R(T)$ at superconducting side (see Fig. S6c) the conductance $G(T)$ in the insulating regime – shown for different magnetic fields in Fig. S6f – displays a maximum that shifts from 0.3 K to 0.5 K from the lowest to the highest field. All curves converge at higher temperatures where the magnetoresistance of the sample becomes small.

## CONCLUSIONS

We have demonstrated that the regime of thermal fluctuations is described with reasonable parameters by the Langer-Ambegaokar model. Both in the superconducting and in the insulating regime our data can be consistently interpreted in terms of the IZ-theory while using very plausible parameters. We find a clear distinction between the more conventional behavior of the wider strips and the unusual reentrant insulation in the narrow strips described in the main text. The magnetoresistance of the most insulating device shows a pronounced peak around 2 T with smaller fluctuations superimposed.

[1] V. Ambegaokar and B. I. Halperin, Phys. Rev. Lett. **22**, 1364 (1969).
[2] D. E. McCumber, J. Appl. Phys. **39**, 3113 (1968).
[3] M. Tinkham, *Introduction to Superconductivity*, 2nd ed. (Dover Publications, Mineola, 1996).
[4] S. V. Postolova, A. Y. Mironov, and T. I. Baturina, JETP Lett. **100**, 635 (2014).
[5] I. V. Zolochevski, Low Temperature Physics **40**, 867 (2014).
[6] H. J. Kim and A. Rogachev, Phys. Rev. B **94**, 245436 (2016).
[7] P. A. Lee and A. D. Stone, Phys. Rev. Lett. **55**, 1622 (1985).
[8] F. L. Vernon and R. J. Pedersen, Journal of Applied Physics **39**, 2661 (1968).
[9] W. J. Skocpol, M. R. Beasley, and M. Tinkham, Journal of Applied Physics **45**, 4054 (1974).
[10] K. Kronfeldner, et al., Unpublished.
[11] Y. M. Ivanchenko and L. A. Zil'berman, Sov. Phys. JETP **28**, 1272 (1969).
[12] J. S. Lehtinen, K. Zakharov, and K. Y. Arutyunov, Phys. Rev. Lett. **109**, 187001 (2012).
[13] C. H. Webster, J. C. Fenton, T. T. Hongisto, S. P. Giblin, A. B. Zorin, and P. A. Warburton, Phys. Rev. B **87**, 144510 (2013).
[14] T. T. Hongisto and A. B. Zorin, Phys. Rev. Lett. **108**, 097001 (2012).
[15] D. B. Haviland, K. Andersson, and P. Ågren, J. Low Temp. Phys. **118**, 733 (2000).
[16] D. Haviland, K. Andersson, P. Ågren, J. Johansson, V. Schöllmann, and M. Watanabe, Physica C **352**, 55 (2001).
[17] S. Corlevi, W. Guichard, F. W. D. Hekking, and D. B. Haviland, Phys. Rev. Lett. **97**, 096802 (2006).
[18] A. Ergül, J. Lidmar, J. Johansson, Y. Azizoglu, D. Schaeffer, and D. B. Haviland, New J. Phys. **15**, 095014 (2013).
